# Supplementary material for: InfoMAE: Pair-Efficient Cross-Modal Alignment for Multimodal Time-Series Sensing Signals
Source: arXiv:2504.09707 source file (2025-04-13)
Supplement: Supplementary file 1 [file clustering.tex]

\begin{table}[t!]
\centering
\caption{Clustering Evaluation}
\resizebox{\columnwidth}{!}{%
\begin{tabular}{@{}cccccccccc@{}}
\toprule
\multicolumn{2}{c|}{Dataset} &
  \multicolumn{2}{c|}{MOD} &
  \multicolumn{2}{c|}{ACIDS} &
  \multicolumn{2}{c|}{RealWorld-HAR} &
  \multicolumn{2}{c}{PAMAP2} \\ \midrule
\multicolumn{1}{c|}{Encoder} &
  \multicolumn{1}{c|}{Framework} &
  ARI &
  \multicolumn{1}{c|}{NMI} &
  ARI &
  \multicolumn{1}{c|}{NMI} &
  ARI &
  \multicolumn{1}{c|}{NMI} &
  ARI &
  NMI \\ \midrule
\multicolumn{1}{c|}{\multirow{5}{*}{DeepSense}} &
  \multicolumn{1}{c|}{CMC} &
  \textbf{0.3936 ± 0.0125} &
  \multicolumn{1}{c|}{\textbf{0.5224 ± 0.0206}} &
  0.2926 ± 0.0156 &
  \multicolumn{1}{c|}{0.5833 ± 0.0051} &
  0.2187 ± 0.1094 &
  \multicolumn{1}{c|}{0.4354 ± 0.1713} &
  0.3024 ± 0.0118 &
  0.5063 ± 0.0120 \\
\multicolumn{1}{c|}{} &
  \multicolumn{1}{c|}{Cosmo} &
  0.1384 ± 0.0540 &
  \multicolumn{1}{c|}{0.2552 ± 0.0803} &
  0.5217 ± 0.0074 &
  \multicolumn{1}{c|}{0.6416 ± 0.0184} &
  0.4231 ± 0.2726 &
  \multicolumn{1}{c|}{0.5318 ± 0.2564} &
  0.3583 ± 0.0781 &
  0.5212 ± 0.0671 \\
\multicolumn{1}{c|}{} &
  \multicolumn{1}{c|}{Cocoa} &
  0.3502 ± 0.0184 &
  \multicolumn{1}{c|}{0.4444 ± 0.0135} &
  0.5453 ± 0.0229 &
  \multicolumn{1}{c|}{0.6767 ± 0.0184} &
  0.3385 ± 0.1826 &
  \multicolumn{1}{c|}{0.4792 ± 0.1940} &
  0.3493 ± 0.0230 &
  0.5091 ± 0.0184 \\
\multicolumn{1}{c|}{} &
  \multicolumn{1}{c|}{GMC} &
  0.1982 ± 0.0674 &
  \multicolumn{1}{c|}{0.3925 ± 0.0416} &
  0.2490 ± 0.0403 &
  \multicolumn{1}{c|}{0.5296 ± 0.0150} &
  0.3433 ± 0.1836 &
  \multicolumn{1}{c|}{0.4794 ± 0.1978} &
  0.3078 ± 0.0194 &
  0.5092 ± 0.0221 \\ \cmidrule(l){2-10} 
\multicolumn{1}{c|}{} &
  \multicolumn{1}{c|}{\textbf{FOCAL}} &
  0.3929 ± 0.0222 &
  \multicolumn{1}{c|}{0.5067 ± 0.0226} &
  \textbf{0.5723 ± 0.0440} &
  \multicolumn{1}{c|}{\textbf{0.7213 ± 0.0432}} &
  \textbf{0.4400 ± 0.2465} &
  \multicolumn{1}{c|}{\textbf{0.5545 ± 0.2437}} &
  \textbf{0.4759 ± 0.0695} &
  \textbf{0.6037 ± 0.0558} \\ \midrule
\multicolumn{1}{c|}{\multirow{5}{*}{SW-T}} &
  \multicolumn{1}{c|}{CMC} &
  0.4314 ± 0.2716 &
  \multicolumn{1}{c|}{0.5413 ± 0.2612} &
  0.3604 ± 0.0119 &
  \multicolumn{1}{c|}{0.5881 ± 0.0009} &
  0.4014 ± 0.0528 &
  \multicolumn{1}{c|}{0.5275 ± 0.0532} &
  0.3718 ± 0.0480 &
  0.5562 ± 0.0401 \\
\multicolumn{1}{c|}{} &
  \multicolumn{1}{c|}{Cosmo} &
  0.2865 ± 0.1521 &
  \multicolumn{1}{c|}{0.4140 ± 0.1946} &
  0.4436 ± 0.0145 &
  \multicolumn{1}{c|}{0.5469 ± 0.0015} &
  0.0029 ± 0.0020 &
  \multicolumn{1}{c|}{0.0107 ± 0.0025} &
  0.2425 ± 0.0301 &
  0.3604 ± 0.0347 \\
\multicolumn{1}{c|}{} &
  \multicolumn{1}{c|}{Cocoa} &
  0.4281 ± 0.2314 &
  \multicolumn{1}{c|}{0.5308 ± 0.2405} &
  0.4363 ± 0.0020 &
  \multicolumn{1}{c|}{0.6824 ± 0.0261} &
  0.2487 ± 0.0053 &
  \multicolumn{1}{c|}{0.3897 ± 0.0024} &
  0.3658 ± 0.0540 &
  0.5330 ± 0.0472 \\
\multicolumn{1}{c|}{} &
  \multicolumn{1}{c|}{GMC} &
  0.3973 ± 0.2177 &
  \multicolumn{1}{c|}{0.4940 ± 0.2184} &
  0.2055 ± 0.0029 &
  \multicolumn{1}{c|}{0.4971 ± 0.0066} &
  0.3050 ± 0.0076 &
  \multicolumn{1}{c|}{0.4342 ± 0.0052} &
  0.2794 ± 0.0206 &
  0.5044 ± 0.0329 \\ \cmidrule(l){2-10} 
\multicolumn{1}{c|}{} &
  \multicolumn{1}{c|}{\textbf{\model}} &
  \textbf{0.4660 ± 0.2737} &
  \multicolumn{1}{c|}{\textbf{0.5693 ± 0.2579}} &
  \textbf{0.6050 ± 0.1027} &
  \multicolumn{1}{c|}{\textbf{0.7389 ± 0.0774}} &
  \textbf{0.4319 ± 0.0851} &
  \multicolumn{1}{c|}{\textbf{0.5462 ± 0.0717}} &
  \textbf{0.4785 ± 0.0914} &
  \textbf{0.6130 ± 0.0730} \\ \bottomrule
\end{tabular}%
}
\label{tab:clustering}
\end{table}
