# Supplementary material for: InfoMAE: Pair-Efficient Cross-Modal Alignment for Multimodal Time-Series Sensing Signals
Source: arXiv:2504.09707 source file (2025-04-13)
Supplement: Supplementary file 2 [file training.tex]

\begin{table*}[]
\centering
\caption{Training configurations.}
\label{tab:appendix_training}
\resizebox{0.85\textwidth}{!}{%
\begin{tabular}{@{}c|c|c|c|c@{}}
\toprule
       & Joint Multimodal Pretraining                                                           & Unimodal Pretraining & Cross-Modal Alignment & Finetuning \\ \midrule
Optimizer                & AdamW \cite{loshchilov2018decoupled}  & AdamW \cite{loshchilov2018decoupled}  & AdamW \cite{loshchilov2018decoupled}  & Adam \cite{kingma2015adam} \\
Weight Decay             & 0.05   & 0.05   & 0.05   & 0.05 \\
Start Learning Rate (LR) & 0.0001 & 0.0001 & 0.0001 & 0.01 \\
LR Scheduler             & Cosine & Cosine & Cosine & Step \\
LR Decay                 & 0.2    & 0.2    & 0.2    & 0.2  \\
LR Period                & 500    & 500    & 100    & 50   \\
Epochs & \begin{tabular}[c]{@{}c@{}}MOD, ACIDS: 2500\\ RealWorld-HAR, PAMAP2: 1000\end{tabular} & 2500                 & 500                  & 200        \\
Batch Size               & 256    & 256    & 256    & 128  \\ \bottomrule
\end{tabular}%
}
\end{table*}

\begin{table*}[!t]
\caption{Discriminator configurations.}
\label{tab:appendix_dis_config}
\centering
\resizebox{0.6\textwidth}{!}{
\begin{tabular}{@{}c|cccc@{}}
\toprule
Dataset             & MOD                     & ACIDS     & RealWorld-HAR & PAMAP2    \\ \midrule
Dropout Ratio       & 0.2                     & 0.2       & 0.2           & 0.2       \\
Mod Conv Kernel     & aud: [1, 5], sei: [1,3] & [1,4]     & [1, 3]        & [1, 5]    \\
Mod Conv Channel    & 128                     & 128       & 128           & 64        \\
Mod Conv Layers     & 5                       & 6         & 6             & 4         \\
MLP Layers          & 4                       & 4         & 4             & 4         \\
Activation Function & LeakyReLU               & LeakyReLU & LeakyReLU     & LeakyReLU \\ \bottomrule
\end{tabular}%
}
\vspace{-0.cm}
\end{table*}

\begin{table}[]
\centering
\caption{Discriminator training configurations.}
\label{tab:appendix_dis_training}
\resizebox{0.5\textwidth}{!}{%
\begin{tabular}{@{}c|c|c@{}}
\toprule
Stage                        & Joint Multimodal Pretraining         & Cross-Modal Alignment                 \\ \midrule
Optimizer      & AdamW \cite{loshchilov2018decoupled} & AdamW \cite{loshchilov2018decoupled} \\
Weight Decay   & 0.005                                & 0.005                                \\
Start LR       & 0.00005                              & 0.00005                              \\
LR Scheduler   & Cosine \cite{loshchilov2017sgdr}     & Cosine \cite{loshchilov2017sgdr}     \\
LR Decay Epochs &
  \begin{tabular}[c]{@{}c@{}}MOD, ACIDS: 500\\ RealWorld-HAR, PAMAP2: 50\end{tabular} &
  \begin{tabular}[c]{@{}c@{}}MOD, ACIDS: 500\\ RealWorld-HAR, PAMAP2: 50\end{tabular} \\
Warm Up Epochs & 10                                   & 10                                   \\
Train Period   & 50                                   & 50                                   \\ \bottomrule
\end{tabular}%
}
\end{table}
