# Supplementary material for: InfoMAE: Pair-Efficient Cross-Modal Alignment for Multimodal Time-Series Sensing Signals
Source: arXiv:2504.09707 source file (2025-04-13)
Supplement: Supplementary file 4 [file discriminator_config.tex]

\begin{table*}[!t]
\caption{Discriminator configurations.}
\label{tab:appendix_dis_config}
\centering
\resizebox{0.6\textwidth}{!}{
\begin{tabular}{@{}c|cccc@{}}
\toprule
Dataset             & MOD                     & ACIDS     & RealWorld-HAR & PAMAP2    \\ \midrule
Dropout Ratio       & 0.2                     & 0.2       & 0.2           & 0.2       \\
Mod Conv Kernel     & aud: [1, 5], sei: [1,3] & [1,4]     & [1, 3]        & [1, 5]    \\
Mod Conv Channel    & 128                     & 128       & 128           & 64        \\
Mod Conv Layers     & 5                       & 6         & 6             & 4         \\
MLP Layers          & 4                       & 4         & 4             & 4         \\
Activation Function & LeakyReLU               & LeakyReLU & LeakyReLU     & LeakyReLU \\ \bottomrule
\end{tabular}%
}
\vspace{-0.cm}
\end{table*}
