# Supplementary material for: InfoMAE: Pair-Efficient Cross-Modal Alignment for Multimodal Time-Series Sensing Signals
Source: arXiv:2504.09707 source file (2025-04-13)
Supplement: Supplementary file 5 [file model_config.tex]

% \begin{table*}[t!]
% \centering
% \caption{Encoder \& Decoder configurations.}
% \label{tab:model_config}
% \resizebox{0.75\textwidth}{!}{%
% \begin{tabular}{@{}c|cccc@{}}
% \toprule
% Dataset                 & MOD                      & ACIDS          & RealWorld-HAR & PAMAP2        \\ \midrule
% Dropout Ratio           & 0.2                      & 0.2            & 0.2           & 0.2           \\
% Patch Size              & aud: [1, 40], sei: [1,1] & [1, 8]         & [1, 2]        & [1, 2]        \\
% Window Size             & [3, 3]                   & [2,4]          & [3, 3]        & [3, 5]        \\
% Encoder Block Num       & [2, 2, 4]                & [2, 2, 4]      & [2, 2, 2]     & [2, 2, 2]     \\
% Encoder Block Channels  & [64, 128, 256]           & [64, 128, 256] & [32, 64, 128] & [32, 64, 128] \\
% Head Num                & 4                        & 4              & 4             & 4             \\
% Encoder Fusion Channel  & 256                      & 256            & 128           & 128           \\
% Encoder Fusion Head Num & 4                        & 4              & 4             & 4             \\
% Encoder Fusion Block    & 2                        & 2              & 2             & 2             \\
% FC Dim                  & 512                      & 512            & 256           & 128           \\
% Factorization Dimension & 128                      & 128            & 128           & 128           \\
% Decoder Block Num       & [2, 2]                   & [2, 2]         & [2, 2]        & [2, 2]        \\
% Decoder Block Channels  & [128, 64]                & [128, 64]      & [64, 32]      & [64, 32]      \\ \bottomrule
% \end{tabular}%
% }
% \end{table*}
