# Supplementary material for: InfoMAE: Pair-Efficient Cross-Modal Alignment for Multimodal Time-Series Sensing Signals
Source: arXiv:2504.09707 source file (2025-04-13)
Supplement: Supplementary file 6 [file additional_downstream.tex]

\begin{table*}[t!]
\centering
\caption{Performance on additional tasks within the MOD dataset.}
% \yatong{Do SimCLR and MoCo get the same results? -> Yes}
\label{tab:additional_task}
\resizebox{0.65\textwidth}{!}{%
\begin{tabular}{@{}cc|cccc@{}}
\toprule
\multicolumn{2}{c|}{Dataset}                           & \multicolumn{4}{c}{MOD}                                                                                \\ \midrule
\multicolumn{1}{c|}{\multirow{2}{*}{Encoder}} & \multirow{2}{*}{Frameworks} & \multicolumn{2}{c|}{Distance Classification} & \multicolumn{2}{c}{Speed Classification} \\
\multicolumn{1}{c|}{}                       &          & Acc             & \multicolumn{1}{c|}{F1}              & Acc                   & F1                    \\ \midrule
\multicolumn{1}{c|}{\multirow{11}{*}{SW-T}} & SimCLR   & 0.9090          & \multicolumn{1}{c|}{0.8694}          & 0.5511                & 0.5514                \\
\multicolumn{1}{c|}{}                       & MoCo     & 0.9090          & \multicolumn{1}{c|}{0.8694}          & 0.6108                & {\ul \textit{0.6105}} \\ \cmidrule(l){2-6} 
\multicolumn{1}{c|}{}                       & CMC      & 0.8180          & \multicolumn{1}{c|}{0.7507}          & 0.5170                & 0.5175                \\
\multicolumn{1}{c|}{}                       & GMC      & 0.8181          & \multicolumn{1}{c|}{0.7450}          & 0.4460                & 0.4405                \\
\multicolumn{1}{c|}{}                       & FOCAL    & \textbf{0.9849} & \multicolumn{1}{c|}{\textbf{0.9726}} & \textbf{0.8329}       & \textbf{0.6920}       \\ \cmidrule(l){2-6} 
\multicolumn{1}{c|}{}                       & TNC      & 0.8484          & \multicolumn{1}{c|}{0.8015}          & 0.4375                & 0.4322                \\
\multicolumn{1}{c|}{}                       & TS-TCC   & 0.7878          & \multicolumn{1}{c|}{0.6575}          & 0.5284                & 0.5230                \\ \cmidrule(l){2-6} 
\multicolumn{1}{c|}{}                       & MMAE     & 0.7272          & \multicolumn{1}{c|}{0.4917}          & 0.4545                & 0.4383                \\
\multicolumn{1}{c|}{}                       & CAV-MAE  & 0.XXX     & \multicolumn{1}{c|}{0.XXX}     & 0.XXX           & 0.XXX           \\
\multicolumn{1}{c|}{}                       & MultiMAE & 0.XXX     & \multicolumn{1}{c|}{0.XXX}     & 0.XXX           & 0.XXX           \\ \cmidrule(l){2-6} 
\multicolumn{1}{c|}{}                       & InfoMAE  & \textbf{0.9849} & \multicolumn{1}{c|}{\textbf{0.9726}} & {\ul \textit{0.8002}} & 0.6056                \\ \bottomrule
\end{tabular}%
}
\end{table*}
